# Supplementary material for: Symbolic Path-guided Test Cases for Models with Data and Time
Source: arXiv:2309.06840 source file (2023-09-13)
Supplement: Supplementary file 1 [file appendix.tex]

%\mskip

%We first characterize a System Under Test. Then, we present TIOCO, a conformance relation relating the correctness of a given timed trace resulting from the execution of a System Under Test against a reference TIOSTS model.
% This relation reasons on traces resulting from the real execution of an LUT and it is these traces that will be called by the LUT and a higher level, more abstract reference model whose semantics is given by traces

\medskip

\noindent We propose to deal with {\bf Localized System Under Test (LUT)} in some distributed context following approaches~\cite{GastonHG13,BGHLG17}. Thus, we need to distinguish between inputs locally received from some users (e.g., an ATM client or test case) and inputs received from other systems (e.g. a distant bank), via the network.

Let us partition $C^{in}$ $C^{in} = CC^{in} \amalg UC^{in}$ where $CC^{in}$ is 
the set of controllable input channels and $UC^{in}$ is the set of uncontrollable input channels. %A channel in $CC^{in}$ is used to receive messages from the test case (hence controllable for the test case), whereas a channel in $UC^{in}$ is used to receive messages emitted by other subsystems (uncontrollable for the test case).
% \commental{ Et c'est quoi la définition informelle (en une demi phase chacune) de ces deux nouvelles notions }

 %We recall that to represent this situation, we introduced in Section \ref{subsec:enrichment_quiescence} the symbol $\_$ to denote the absence of reaction observed by the tester. 

%It might happen that the test case does not wait long enough to observe a reaction of a LUT because the delay is not known in advance (and in whole generality not bounded).

We denote by $Evt(C)=M_{time} \times (Act(C) \cup \{\_\})$ the set of all concrete events that occur in trace. For any $ev = (d,act) \in Evt(C)$, $delay(ev)$ and $act(ev)$ denote resp. $d$ and $act$. We distinguish $Evt(\{\_\}) \subseteq Evt(C)$ the set of events of the form  $(d, \_)$ that will be used to denote that after waiting delay $d$, no reaction of LUT is observed. $\overline{Evt}(C)$ stands for $Evt(C) \setminus Evt(\{\_\})$.

A LUT is as a black box, and therefore can be abstracted by a set of traces $LUT \subseteq Evt(C)^*$ satisfying the following additional hypotheses. For any traces $\sigma_1, \sigma_2 \in \overline{Evt}(C)^*$ and event $ev \in \overline{Evt}(C)$, we have that :

\begin{itemize}
    \item stable by prefix: $$\sigma_1.\sigma_2\in LUT \Rightarrow \sigma_1\in LUT$$
    
    \item quiescence: for any $d<delay(ev)$, 
    
    $$\sigma_1 .ev\in LUT \Rightarrow \sigma_1 .(d,\_)\in LUT$$
    
    \item input complete:  for any $d<delay(ev)$, $c\in CC^{in}$, $v\in M$, 
    
    $$\sigma_1 .ev\in LUT \Rightarrow \sigma_1 .(d,c?v)\in LUT$$
\end{itemize}

The hypothesis on quiescence states that if the LUT is waiting for an event $ev$ whose action is not empty, then any duration which is strictly less than the delay of $ev$ is accepted by the LUT. The hypothesis on input completeness enables LUT to receive any input on a controllable channel, i.e. an input received from the test cases, during the delay of $ev$.

% In the following, we present tioco, timed conformance relation between a timed trace of the LUT and timed traces that can be generated from the reference model. 

% \commental{ manque une reférence pour justifier ou UNE INTRO de la section 3.2 \label{sec:timed_conformance_relation}, genre la description ( résumé ) informelle d'un process chapeau ou intervient le LUT
% \newline
% Pour la définition/présentation de TIOCO, on a besoin de quelques préliminaires... le LUT qui est ...
% \newline
% Etc.
% }

\noindent {\bf Timed Input Output Conformance relation (TIOCO)} In order to reflect the quiescence situations that can be observed during the test execution on $LUT$, we define the semantics of $\mathbb{G}$, denoted by $Sem(\mathbb{G})$, as the smallest set containing ${Traces}(\mathbb{G})$ and such that for any $\sigma \in \overline{Evt}(C)^*$, $ev\in \overline{Evt}(C)$, for any $d<delay(ev)$: 
$$\sigma.ev\in Traces(\mathbb{G}) \Rightarrow \sigma .(d,\_)\in Sem(\mathbb{G})$$ 

% \commental{Difference entre $Trace(\mathbb{G})$ et $Sem(\mathbb{G}$ : bien expliquer au chapitre précédent ???? rappel informel en une phrase ? }

% We stress that, as a consequence of (distributed?) TIOSTS semantics,  when $\mathbb{G}$ is waiting for an event $ev$, it accepts any duration which is strictly less than the delay of $ev$.

Consequently, when $\mathbb{G}$ is waiting for an event $ev$, it accepts any duration which is strictly less than the delay of $ev$.

% The semantics of a TIOSTS $\mathbb{G}$ can be seen as timed traces (cf Section \ref{subsec:Semantics_TIOSTS}). 

% A timed trace $\sigma$ is a sequence $(d_1, act_1) \ldots (d_n, act_n)$ where $(d_i, act_i)$ is called an \textit{event} which constitutes a concrete communication action $act_i \in Act(C)$ and $d_i \in D_+$ the time elapsed between the two actions $act_{i-1}$ and $act_i$ (where $D^+$ is the set of strictly positive real numbers). In the remainder, for an event $ev$ of the form $(d, act)$, we denote $delay(ev)$ the delay $d$ and $act(ev)$ the action $act$. The set of events is denoted as $Evt(C)$.

% \commental{Comment peut-on passer de cette propriété  $LUT \subseteq (Evt(C) \cup Evt(\{\_\}))^*$ vu sous la notation précédence à la caractérisation par un TIOSTS sans aucune phrase de liaison ! AU MOIN PARLER DE REPRESENTATION NATURELLE / CANONIQUE des 3 itemps par un TIOSTS }.

We use the following reformulation of the TIOCO relation~\cite{KrichenT04} : 
%to define correctness of a LUT with respect to a TIOSTS $\mathbb{G}$:
 
LUT tioco $\mathbb{G}$ if and only if, for all $\sigma \in Sem(\mathbb{G})$, for any either event $ev\in \overline{Evt}(C)$ with $chan(ev)\in C^{out}$ or $ev\in Evt(\{\_\})$, we have:

$$\sigma.ev \in LUT \Rightarrow \sigma.ev\in Sem(\mathbb{G})$$

TIOCO states that the LUT is in conformance with the TIOSTS model, if and only if after a specified sequence of events between the LUT and the test case, any event produced by the LUT either a reaction or an observation of a delay, must be specified in the reference model.

\medskip

\textcolor{red}{ === BB: JE SUIS LA ========}

\noindent {\bf Test case generation} can be based on the selection of a test purpose which permits to characterize a particular behavior in the reference model to be tested~\cite{AndradeMJM11,BannourEGG12,HesselLMNPS08}. Our test purpose is a path $tp=ec_0ec_1\ldots ec_n \in SPaths(\mathbb{G})$ that is guided in practice by a non-empty consecutive sequence of TIOSTS transitions $tr_1 \ldots tr_n \in Tr^+$, i.e., we have $tr_i=tr(ec_i)$ for $i\in [1,n]$. To simplify the test case definition, we consider only deterministic reference TIOSTS so that some execution is exclusively inside the test purpose or outside of it.

%For any decomposition of $tp = ec_0 ec_1 \ldots ec_i \ldots ec_n$,  $pre(ec_i)$ refers to the sequence of ECs occurring before $ec_i$ while $post(ec_i)$ refers to the sequence of ECs occurring after $ec_i$ in $tp$.

%\end{notation}

% \commental{ Et là pour digérer la suite , j'aurai aimé un exemple concret avec une vraie trace symbolique et une illustration concrète des différentes variantes de $Fresh(ec)$ ! 
% \newline BREF SPOILER LA TRACE EC1...EC6 si justement utilisée dans la suite
% \newline $tp$ pour Test Purpose et $sp$ pour Symbolic Path ? si oui le dire ! mais symbolic path c'est déjà $p$ ! Je suis perdu là
% }

The process of test case generation will be applied to a fully-prepared symbolic tree containing ECs of the test purpose $tp$ and adjacent ECs. These are successors of the ECs inside $tp$. Typically, this is the case of the symbolic tree of the Fig.~\ref{def:tiosts-symbex} for $tp=ec_0 ec_1 \ldots ec_5$. 

In addition, we consider a global maximal waiting-time denoted as a constant $\maxWaitingBound$, in order to bound the waiting delay for observing outputs or internal inputs emitted by other systems. The waiting-time fixed in the test case to avoid waiting for too long for such observations. For instance, it can be chosen as the maximal value among those which bound the occurrences of observations (if any) in the definition of the test purpose, plus some duration. 

We generate a test case in the form of a (deterministic) TIOSTS $\mathbb{G}_{\tc}=(Q_{\tc}, {q_0}_{\tc}, Tr_{\tc})$ over a signature $\Sigma_{\tc} = (A_{\tc}, K_{\tc}, C_{\tc})$ defined partially based on the signature $\Sigma_F = (F, \emptyset, C)$ of the symbolic execution of the reference TIOSTS $\mathbb{G}$ as follows:

\begin{itemize}
    \item $A_{\tc} = f(tp)\setminus f(tgt(tp))$ is the set of fresh variables used to compute $tp$;

\item $K_{\tc}=\{\tclk\}$ with $\tclk$ measures the delay of events in the test case;

\item $C_{\tc}=C$ is such that ${(C_{\tc})}^{in} = C^{out} \cup UC^{in}$ and ${(C_{\tc})}^{out} = CC^{in}$

    \item $Q_{\tc} = \mathbb{V} \cup \big(\mathbb{EC}(tp) \setminus \{tgt(tp)\} \big)$ where
    
    $\mathbb{V}=\{\text{PASS}, \text{FAIL}_{out},\text{FAIL}_{time},\text{INC}_{out},\text{INC}_{time},\text{INC}_{specIntI},\text{INC}_{uspecIntI}\}$ is the set of states of test verdicts, and $\mathbb{EC}(tp)$ is the set of states inside $tp$ form which $tgt(tp)$ is excluded as replaced by $\text{PASS}\in \mathbb{V}$;
    
    \item ${q_0}_{\tc}=ec_0$ being the initial context from which $tp$ is computed;
    
    \item $Tr_{\tc}$ is defined as follows.
    
\end{itemize}

Let us construct the test case transitions $tr_{\tc}$ by considering $ec$ in the test purpose.

\medskip

 {\bf R1 - stimulation:} Case $ev(ec) = (z,c?x_c)$ with $c \in CC^{in}$, we build the following transition

\[tr_{\tc}=\big( q_{pec(ec)},c!x_c, \tclk = z \wedge \wedge \exists (F^{ini} \cup Var(\pi(tp)) ) \setminus pf(ec). \pi(tp) , \{\tclk\} , \langle \rangle,q_{ec} \big) \]

{\bf R2 - authorized reaction inside $tp$:} Case $ev(ec)=(z,c!y_c)$, the ingredients of $tr_{\tc}$ in this case are:

\builtTransitionAlt
    {$q_{pec(ec)}$} % source
    {$\{\tclk\}$}    % clock  if $post(ec) \neq \epsilon$
    {$\emptyset$} % clock else
    {$\tclk < \maxWaitingBound \land \tclk = z  \bigwedge \exists F^{ini}.\pi(ec)$} % guard
    {$c?y_c$} % action
    {$\big\langle ~\big\rangle$} % substitution
    {$q_{ec}$} % target $post(ec) \neq \epsilon$
    {$Pass$}   % target else

% 	if $post(ec)=\epsilon$ then $tgt(tr)=q_{ec}$ is further substituted by $Pass$ and $Clk(tr)$ is substituted by $\emptyset$
	
	 \noindent N.B., we denote $\widetilde{\phi}(tr_{\tc}) = \exists F^{ini}.\neg \pi(ec)$. The construction of $\widetilde{\phi}(tr_{\tc})$ is necessary for constructing transitions by R4.

  \medskip

{\bf R3 - authorized reaction outside $tp$:} In case there exists $ec'\neq ec$ such that $pec(ec')=pec(ec)$ and $ev(ec')=(z,c!y_c)$,

% \commental{Il faudrait, d'une manière ou d'une autre, préciser que le $ec$ auquel on fait référence avec $pec(ec)$ est bien le ec de la dernière règle R2 appliquée selon ton process défini en préliminaire ! Mais peut être que le <<w.r.t. our process>> un peut plus bas suffit}

\builtTransition
    {$q_{pec(ec)}$} % source
    {$\emptyset$} % clock
    {$\tclk < \maxWaitingBound \land \tclk = z  \bigwedge \exists F^{ini}.\pi(ec')$} % guard
    {$c?y_c$} % action
    {$\big\langle ~\big\rangle$} % substitution
    {$Inc_{out}$} % target
	
    %\noindent N.B., we denote $\widetilde{\phi}(tr)$, the formula obtained by omitting the formulas $\tclk < \maxWaitingBound$ and $cl = z$ in $\phi(tr)$. \\
    
    \noindent N.B., we denote $\widetilde{\phi}(tr_{\tc}) = \exists F^{ini}.\neg \pi(ec')$. The construction of $\widetilde{\phi}(tr_{\tc})$ is necessary for constructing transitions by R4.

  \medskip

 {\bf R4 - unauthorized reaction:}
% \commental{Au regard de ce qui est autorisé par R2 (au sens ou on vient d'appliquer R2), toujours w.r.t. our process}

\builtTransition
    {$q_{ec}$} % source 
    {$\emptyset$} % clock
    {$\tclk < \maxWaitingBound \land \tclk = f^{dur}(ec) \bigwedge_{\substack{tr' \in Tr'}} 
	\widetilde{\phi}(tr')$} % guard
    {$c?f^{out}_c(ec)$} % action
    {$\big\langle ~\big\rangle$} % substitution
    {$Fail_{out}$} % target
   
    Where $Tr'$ is the set $\{ tr' \;\; | \;\; tr' \in Tr_{\tc} \wedge src(tr') = q_{ec} \wedge tgt(tr') \neq Fail_{out} \wedge act(tr')=c?f^{out}_c(ec)\}$ and 
    $\widetilde{\phi}(tr')$ is the formula defined in R2 and R3. \\
    % $\neg(\exists_{IFresh(ec_1) \setminus PFresh(ec)} (OCond(ec) \land \pi(ec)))$. \\

\medskip {\bf R5 - internal input inside $tp$:} Case $ev(ec)=(z,c?x_c)$ and $c\in UC^{in}$, we build the following transition

\builtTransitionAlt
    {$q_{pec(ec)}$} % source
    {$\{\tclk\}$}      % clock if {$post(ec) \neq \epsilon$}
    {$\emptyset$}   % clock else
    {$\tclk < \maxWaitingBound \land \tclk= z \bigwedge \exists F^{ini} .\pi(ec)$} % guard
    {$c?x_c$} % action
    {$\big\langle ~\big\rangle$} % substitution
    {$q_{ec}$}       % target if $post(ec) \neq \epsilon$
    {$Pass$}         % target else

% 	if $post(ec)=\epsilon$ then $tgt(tr)=q_{ec}$ is further substituted by $Pass$, and $Clk(tr)$ is substituted by $\emptyset$
	
	N.B., we denote $\widetilde{\phi}(tr_{\tc}) = \exists F^{ini}.\neg \pi(ec')$. The construction of $\widetilde{\phi}(tr_{\tc})$ is necessary for constructing transitions by R7.

 \medskip

{\bf R6 - internal input outside $tp$:} In case there exists $ec'\neq ec$ such that $pec(ec')=pec(ec)$ and $ev(ec')=(z,c?x)$, $c\in UC^{in}$:

	\builtTransition
    {$q_{pec(ec)}$} % source
    {$\emptyset$} % clock
    {$\tclk < \maxWaitingBound \land \tclk= z \bigwedge \exists F^{ini} .\pi(ec')$} % guard
    {$c?OFresh(pec(ec))_c$} % action
    {$\big\langle ~\big\rangle$} % substitution
    {$Inc_{specIntI}$} % target
	
   \noindent N.B., we denote $\widetilde{\phi}(tr_{\tc})= \exists F^{ini} .\neg \pi(ec')$. The construction of $\widetilde{\phi}(tr_{\tc})$ is necessary for constructing transitions by R7.

\medskip 

{\bf R7 - under-specified internal input:}

    \builtTransition
    {$q_{ec}$} % source
    {$\emptyset$} % clock
    {$\tclk < \maxWaitingBound \land \tclk = f^{dur}(ec) \bigwedge_{tr' \in Tr'} \widetilde{\phi}(tr')$} % guard
    {$c?f^{in}_c(ec)$} % action
    {$\big\langle ~\big\rangle$} % substitution
    {$Inc_{uspecIntI}$} % target
   
    Where $Tr'$ is the set $\{ tr' \;\; | \;\; tr' \in Tr_{\tc} \wedge src(tr') = q_{ec} \wedge tgt(tr')\neq Inc_{uspecIntI} \wedge act(tr')=c?f^{in}_c(ec) \}$ \\
    and $\widetilde{\phi}(tr')$ is the formula defined in R5 and R6. \\

\medskip

{\bf R8 - authorized quiescence on bound $\maxWaitingBound$ ($\maxWaitingBound$ is the max. waiting-time for observations)}: Case $ec$ such that there exists $ec'$ satisfying $pec(ec')=ec$ and $chan(ec)\in (C^{out} \cup UC^{in})$,

    \builtTransition
    {$q_{ec}$} % source
    {$\emptyset$} % clock
    {$\tclk \geq \maxWaitingBound \land \tclk= f^{dur}(ec) \bigwedge 
	(\phi_\delta \vee \phi_{out} \vee \phi_{intI})$} % guard
    {$\_$} % action
    {$\big\langle ~\big\rangle$} % substitution
    {$Inc_{time}$} % target
	
	N.B., $\phi_\delta=\bigwedge_{ec'\in React(ec)}( \forall F^{ini}.(\forall_{z}(\neg\pi(ec'))))$, where $z=f^{dur}(ec)$ ($f^{dur}(ec)$ is the fresh duration introduced to represent the time elapsed from $ec$, and finally $React(ec)=\{ec' \; | \; pec(ec')=ec \wedge chan(ec')\in C^{out}\}$

	$\phi_{out}=\bigvee_{ec'\in React(ec)} \exists F^{ini}.\pi(ec')$,
	
	$\phi_{intI}=\bigvee_{ec'\in Uncont(ec)} \exists F^{ini} .\pi(ec')$,
	
	where $Uncont(ec)=\{ec' \; | \; pec(ec')=ec \wedge chan(ec')\in UC^{in}\}$\\

\medskip 

{\bf R9 - unauthorized quiescence on bound $\maxWaitingBound$ ($\maxWaitingBound$ is the max. waiting-time for observations)}: Case $ec$ such that exists $ec'$ satisfying $pec(ec')=ec$ and $chan(ec)\in (C^{out} \cup UC^{in})$,

    \builtTransition
    {$q_{ec}$} % source
    {$\emptyset$} % clock
    {$\tclk \geq \maxWaitingBound \land \tclk= f^{dur}(ec) \bigwedge 
	(\neg \phi_{out} \land \neg \phi_{intI} )$} % guard
    {$\_$} % action
    {$\big\langle ~\big\rangle$} % substitution
    {$Fail_{time}$} % target

	we remark that $\neg\phi_\delta=\bigvee_{ec'\in React(ec)}( \exists F^{ini} . \exists z.\pi(ec') )$ captures exactly the situation when a duration is compatible with a reaction which is still possible to come, it is omitted as it contradicts the targeted verdict here, fail due to non-conforming duration.
