# Supplementary material for: Symbolic Path-guided Test Cases for Models with Data and Time
Source: arXiv:2309.06840 source file (2023-09-13)
Supplement: Supplementary file 3 [file proof_old0.tex]

\section*{Proof}

\noindent Let us prove Th.\ref{th:corr} by using the contraposition principle. This means to prove that if there such transition exists $tp$ and test case $\mathbb{TC}$ for $tp$ such that $FAIL^{out},FAIL^{dur}\in vdt(LUT, \mathbb{TC})$ then $\neg(LUT~tioco~\mathbb{G})$. Based on the TIOCO definition, the non-conformance $\neg(LUT~tioco~\mathbb{G})$ amounts to prove that there exists $\sigma \in Sem(SE(G)^\delta) \cap LUT$, and an $ev\in Evt(C^{out} \cup \{\delta\})$ such that : $\sigma.ev \in LUT$ and $\sigma.ev\not\in Sem(SE(G)^\delta)$. This is proved by the following proposition.

\begin{proposition}
\label{prop:corr}
If if there such transition exists $tp$ and test case $\mathbb{TC}$ for $tp$ such that 

$(\sigma.ev.\sigma',{q_{\text{TC}}}_0, \nu) ~\overset{*}{\leadsto}_{\mathbb{TC}} (\sigma',\text{Verdict}, \nu' )$ with $\text{Verdict} \in \{\text{FAIL}^{out},\text{FAIL}^{dur}\}$~:

\begin{enumerate}

\item $ev\in Evt(C^{out} \cup \{\delta\})$

\item $\sigma \in Sem(SE(G)^\delta)\cap LUT$ 

\item $\sigma.ev\in LUT$

\item $\sigma.ev\not\in Sem(SE(G)^\delta)$
\end{enumerate}
\end{proposition}

{\bf{\em Proof of (2) in Prop.\ref{prop:corr}}} 

$\sigma \in LUT$ is a hypothesis as the execution relation applies on $LUT$ traces. Let us prove $\sigma \in Sem(SE(G)^\delta)$. 

As  $(\sigma.ev.\sigma',{q_{\text{TC}}}_0, \nu) ~\overset{*}{\leadsto}_{\mathbb{TC}} (\sigma',\text{Verdict}, \nu' )$ with $\text{Verdict} \in \{\text{FAIL}^{out},\text{FAIL}^{dur}\}$, we can state that the last execution step until just before the consumption of $ev$ does not lead to a verdict, i.e. we have decomposition $(\sigma.ev.\sigma',{q_{\text{TC}}}_0, \nu) ~\overset{*}{\leadsto}_{\mathbb{TC}} (ev.\sigma',q, \nu_1 ) \leadsto_{\mathbb{TC}} (\sigma',\text{Verdict}, \nu' )$ with $q\not\in \mathbb{V}$. This because the Test Case transition (TC-transition in short) that corresponds to the step of execution of $ev$ has as source an execution context and not a verdict by definition of rule $R5\; \text{FAIL}^{our}$ or rule $R10\;\text{FAIL}^{dur}$. 

In addition based on the execution steps and their underlying TC-transitions, we can state that any event in $\sigma$ is either of the form $(d,c!v)$ or $(d,c?v)$, and cannot be of the form $(d,\delta!)$. This because there is no TC-transition $tr$ with target state being an execution context and $chan(tr)=\delta$: Only rule $R9\;\text{INC}^{dur}$ and rule $R10\;\text{FAIL}^{dur}$ produce TC-transition on channel $\delta$ and their target state is a verdict.  



We have now to prove that if $(\sigma.ev.\sigma',{q_{\text{TC}}}_0,\nu) \overset{*}{\leadsto}_{\mathbb{TC}} ( ev.\sigma',q, \nu_1 )$ %with $q\not\in \mathbb{V}$,
then $\sigma \in Sem(SE(G)^\delta)$. We conduct a proof by induction on the size of $\sigma$ as follows.

\medskip 

\noindent Case $\sigma$ of size $1$, i.e., $\sigma=ev_1$, given $(ev_1.ev.\sigma',{q_{\text{TC}}}_0,\nu) \leadsto_{\mathbb{TC}} (ev.\sigma',q, \nu_1 )$, we show that $ev_1\in Sem(SE(G)^\delta)$:

\begin{itemize}
    \item Case $ev_1=(d,c!v)$: If we note $tr$ the TC-transition that allows the execution of $ev_1$ with $chan(tr)=c$ (such transition exists by definition of $\leadsto_{\mathbb{TC}}$) then :  

    we have $tgt(tr)=q$, which is an execution context that we denote $ec$ (i.e., $ec=q$); we have also $ev(ec)=(z,c!y)$ with $z=f ^{dur}(ec_0)$ and $y=f^{out}_c(ec_0)$, where $pec(ec)={q_{\text{TC}}}_0$ which is the initial execution context $ec_0$; and

    \medskip
    
    $\phi(tr) = (z < \maxWaitingBound) \land (\exists F^{ini}.\pi( ec ) ) $  
    
    \hfill(by rule $R2\;\text{SKIP}$).

    \medskip 

   On the other hand $M \models_{\nu_1}  \phi(tr)$ where $\nu_1=\nu[z \mapsto d][y\mapsto v]$ (by definition  $\leadsto_{\mathbb{TC}}$) then $M \models_{\nu_1} \exists F^{ini}.\pi( ec )$ ($\nu_1$ satisfies the right-side of the conjunction of $\phi(tr)$). We can thus compute a trace for the path $p=ec_0ec$ %(a path indeed because $pec(ec)=ec_0$)
   using $\nu_1$, i.e. $\nu_1(p)=\nu_1( (ev(z,c!y) )$ which is $(\nu_1(z),c!\nu_1(y)=(d,c!v))$ equals $ev_1$. We conclude that $ev_1\in Traces(SE(\mathbb{G}^\delta))$ and hence $ev_1 \in Sem(SE(\mathbb{G}^\delta))$.

\medskip 

    \item Case $ev_1=(d,c?v)$ with $c\in UC^{in}$ (similar to $ev_1=(d,c!v)$): If we note $tr$ the TC-transition that allows the execution of $ev_1$ with $chan(tr)=c$ (such transition exists by definition of $\leadsto_{\mathbb{TC}}$) then :  

       we have $tgt(tr)=q$, which is an execution context that we denote $ec$ (i.e., $ec=q$); we have also $ev(ec)=(z,c?x)$ with $z=f ^{dur}(ec_0)$ and $y=f^{in}_c(ec_0)$, where $pec(ec)={q_{\text{TC}}}_0$ which is the initial execution context $ec_0$; and

    \medskip
    
    $\phi(tr) = (z < \maxWaitingBound) \land (\exists F^{ini}.\pi( ec ) ) $  
    
    \hfill(by rule $R6\;\text{SKIP}$).

    \medskip 

   On the other hand $M \models_{\nu_1}  \phi(tr)$ where $\nu_1=\nu[z \mapsto d][x\mapsto v]$ (by definition  $\leadsto_{\mathbb{TC}}$) then $M \models_{\nu_1} \exists F^{ini}.\pi( ec )$ ($\nu_1$ satisfies the right-side of the conjunction of $\phi(tr)$). We can thus compute a trace for the path $p=ec_0ec$ %(a path indeed because $pec(ec)=ec_0$)
   using $\nu_1$, i.e. $\nu_1(p)=\nu_1( (ev(z,c?x) )$ which is $(\nu_1(z),c?\nu_1(x)=(d,c?v))$ equals $ev_1$. We conclude that $ev_1\in Traces(SE(\mathbb{G}^\delta))$ and hence $ev_1 \in Sem(SE(\mathbb{G}^\delta))$.

\medskip 

%STIM
     \item Case $ev_1=(d,c?v)$ with $c\in CC^{in}$: If we note $tr$ the TC-transition that allows the execution of $ev_1$ with $chan(tr)=c$ (such transition exists by definition of $\leadsto_{\mathbb{TC}}$) then :  

       we have $tgt(tr)=q$, which is an execution context that we denote $ec$ (i.e., $ec=q$); we have also $ev(ec)=(z,c?x)$ with $z=f ^{dur}(ec_0)$ and $y=f^{in}_c(ec_0)$, where $pec(ec)={q_{\text{TC}}}_0$ which is the initial execution context $ec_0$; and

    \medskip
    
        $\phi(tr)=(\exists (F^{ini} \cup Var(\pi(tp)) ) \setminus (pf^{dur}(ec) \cup pf^{in} (ec) \cup pf^{out}(ec)). \pi(tp) )$
    
    \hfill(by rule $R1\;\text{SKIP}$).

    \medskip 

   On the other hand $M \models_{\nu_1}  \phi(tr)$ where $\nu_1=\nu[z \mapsto d][x\mapsto v]$ (by definition  $\leadsto_{\mathbb{TC}}$). Given $ec$ is a context of the test purpose $tp$, hence its path condition $\pi(ec)$ is in conjunction some other constraints accumulated until $tgt(tp)$ (by the definition of symbolic execution), then 
   
   $M \models_{\nu_1} \exists (F^{ini} \cup Var(\pi(tp)) ) \setminus (pf^{dur}(ec) \cup pf^{in} (ec) \cup pf^{out}(ec)).\pi( ec )$. 
   
   We have also that $\nu_1$ satisfies $\pi(ec_1)$ for the values $d$ resp. $v$  associated with $f^{dur}(ec_0)$ resp. $f^{in}_c(ec_0)$ through $\nu_1$ because these variables are excluded from the variables which are bound by the existential quantifier in the expression of $\phi(tr)$ ($pf^{dur}(ec)=\{f^{dur}(ec_0)\}$ and $pf^{in}(ec)=\{f^{in}_c(ec_0)\}$). 
   
   
   Given that variables of $Var(tp)$ other than $f^{dur}(ec_0)$, $f^{in}_c(ec_0)$, can be equally considered to be bound or not bound by the existential quantifier in the previous satisfaction statement through $\nu_1$, we have that $M \models_{\nu_1} \exists F^{ini}.\pi( ec )$. We can thus compute a trace for the path $p=ec_0ec$ %(a path indeed because $pec(ec)=ec_0$)
   using $\nu_1$, i.e. $\nu_1(p)=\nu_1( (ev(z,c?x) )$ which is $(\nu_1(z),c?\nu_1(x)=(d,c?v))$ equals $ev_1$. We conclude that $ev_1\in Traces(SE(\mathbb{G}^\delta))$ and hence $ev_1 \in Sem(SE(\mathbb{G}^\delta))$.

    
\end{itemize}
 

\medskip


\noindent Induction case on size of $\sigma$ greater than $1$, i.e., $\sigma=\sigma_*.ev_*$ with $\sigma_*$ non-empty trace, given $(\sigma_*.ev_*.ev.\sigma',{q_{\text{TC}}}_0,\nu)  \overset{*}{\leadsto}_{\mathbb{TC}} (ev_*.ev.\sigma',q_*, \nu_* ) \leadsto_{\mathbb{TC}} (ev.\sigma',q, \nu_1 )$, we show that $\sigma_*.ev_*\in Sem(SE(G)^\delta)$ :


\begin{itemize}

\item Case $ev_*=(d,c!v)$: If we note $tr$ the TC-transition that allows the execution of $ev_*$ with $chan(tr)=c$ (such transition exists by definition of $\leadsto_{\mathbb{TC}}$) then :  

    we have $tgt(tr)=q$, which is an execution context that we denote $ec$ (i.e., $ec=q$); we have also $ev(ec)=(z,c!y)$ with $z=f ^{dur}(ec_*)$ and $y=f^{out}_c(ec_*)$, where $pec(ec)=ec_*$ ($q_*=ec_*$) the predecessor context of $ec$; and

    \medskip
    
    $\phi(tr) = (z < \maxWaitingBound) \land (\exists F^{ini}.\pi( ec ) ) $  
    
    \hfill(by rule $R2\;\text{SKIP}$).

    \medskip 

    By the induction hypothesis, we have that  $\sigma_* \in Sem(SE(\mathbb{G})^\delta)$. Let us reason with the interpretation $\nu_*$ such that $\nu_* \models \exists F^{ini}.\pi(ec_*)$ which allows the computation of $\sigma_*$ carried by some path $p_*$ such that $tgt(p_*)=ec_*$ and $\nu_*(p_*)=\sigma_*$.

   On the other hand $M \models_{\nu_1}  \phi(tr)$ where $\nu_1=\nu_*[z \mapsto d][y\mapsto v]$ (by definition  $\leadsto_{\mathbb{TC}}$) then $M \models_{\nu_1} \exists F^{ini}.\pi( ec )$ ($\nu_1$ satisfies the right-side of the conjunction of $\phi(tr)$). We can thus compute a trace for the path leading to $ec$ using $\nu_1$, i.e. $\nu_1(p)=\nu(p_*).\nu_1( (ev(z,c!y) )$ which is $\sigma_*.(\nu_1(z),c!\nu_1(y)=(d,c!v))$ equals $\sigma_*.ev_*$. We conclude that $\sigma_*.ev_*\in Traces(SE(\mathbb{G}^\delta))$ and hence $\sigma_*.ev_* \in Sem(SE(\mathbb{G}^\delta))$.

\medskip 

\item Cases $ev_*=(d,c?v)$ with $c\in UC^{in}$ and $ev=(c?v)$ with $c\in CC^{in}$ are similar to the previous case. As for previous case of $ev_*=c!v$, the reasoning uses the arguments of the base cases of induction transposed to $ev_*$.
\end{itemize}


\textcolor{red}{ === BB: JE SUIS LA ========}

{\bf{\em Proof of (4) in Prop.\ref{prop:corr}}}

Given the execution $(\sigma.ev.\sigma',{q_{\text{TC}}}_0, \nu) ~\overset{*}{\leadsto}_{\mathbb{TC}} (\sigma',\text{Verdict}, \nu' )$ with $\text{Verdict} \in \{\text{FAIL}^{out},\text{FAIL}^{dur}\}$, we prove that $\sigma.ev\not\in Sem(SE(G)^\delta)$.

\begin{itemize}
   
\item Case of decomposition $(\sigma.ev.\sigma',{q_{\text{TC}}}_0, \nu) ~\overset{*}{\leadsto}_{\mathbb{TC}} (ev.\sigma',q, \nu_1 ) {\leadsto}_{\mathbb{TC}} (\sigma',\text{FAIL}^{out}, \nu' )$:

In this case, we have 
we have that $ev$ is of the form $(d,c!v)$ (by definition  $\leadsto_{\mathbb{TC}}$). 

By {\bf{\em (2) (Prop.\ref{prop:corr}}}), we have that  $\sigma \in Sem(SE(\mathbb{G})^\delta)$. Let us reason with the interpretation $\nu_1$ such that $\nu_1 \models \exists F^{ini}.\pi(ec)$ with $ec=q$ which allows computation of $\sigma$ carried by some path $p$ such that $tgt(p)=ec$ and $\nu_1(p)=\sigma$. 

 We will reason by contradiction. That is let us consider $\sigma.ev \in Sem(SE(\mathbb{G})^\delta)$. Then, there exists an execution context $ec'=pec(ec)$ such that $ev(ec')= (z,c!y)$, $\nu'=\nu_1[z\mapsto d][y\mapsto v]$, and $\nu' \models \exists F^{ini}.\pi(ec')$, $ev(ec')=ev$ {\bf{\em (i)}}.

 %Let us consider $\nu'=\nu_1[z\mapsto d][y\mapsto v]$.

Now if we note $tr$ the TC-transition that allows the execution of $ev$ with $chan(tr)=chan(ev)$ (such transition exists by definition of ${\leadsto}_{\mathbb{TC}}$) then as the verdict is $\text{FAIL}^{out}$, .i.e, $tgt(tr)=\text{FAIL}^{out}$, we have $ev(ec)=c!y$ with $ec=src(tr)$ and $c=chan(ev)\in C^{out}$; and

\medskip

\noindent $\begin{array}{ll}
     \phi(tr) = & (f^{dur} (ec)  < \maxWaitingBound )  \\
      & \land  \bigwedge_{\substack{pec(ec') =ec_1 \\ chan(ec')=c }}(\forall F^{ini}.\neg\pi(ec'))
\end{array}
$ 

 \hfill(by rule $R5\;\text{FAIL}^{out}$).

 %On the other hand $M \models_{\nu_1}  \phi(tr)$ where $\nu_1=\nu[z \mapsto d][x\mapsto v]$ (by definition  $\leadsto_{\mathbb{TC}}$)


On the other hand $\nu'\models \phi(tr) $ thus $\nu' \models (\forall F^{ini}.\neg\pi(ec'))$ where $ec'$ as $ec'=pec(ec_1)$ and $chan(ec')\in C^{out}$ is the one among what figures in the conjunction of $ \phi(tr) $ (ii)

from (i) and (ii) we have contradiction thus $\sigma.ev\not\in Sem(SE(\mathbb{G})^\delta)$


\item Case of decomposition $(\sigma.ev.\sigma',{q_{\text{TC}}}_0, \nu) ~\overset{*}{\leadsto}_{\mathbb{TC}} (ev.\sigma',q_1, \nu_1 ) {\leadsto}_{\mathbb{TC}} (\sigma',\text{FAIL}^{dur}, \nu' )$. 

From {\bf{\em (2) in Prop.\ref{prop:corr}}} we have that  $\sigma \in Sem(SE(\mathbb{G})^\delta)$, 

we can reason with the interpretation $\nu_1$ such that $\nu_1 \models \exists F^{ini}.\pi(ec_1)$ with $ec_1=q_1$ which allowed computation of $\sigma$ carried by some path $p_1$ ($tgt(p_1)=ec_1$, $\nu_1(p_1)=\sigma$).

let us consider $\nu'=\nu_1[z\mapsto d]$
by contradiction, if $\sigma.ev \in Sem(SE(\mathbb{G})^\delta))$ then exists :
\begin{itemize}
    \item $ec'=pec(ec_1)$ s.t. $\nu' \models \exists F^{ini}.\pi(ec')$, $ev(ec')=ev$ (i) as $\sigma.(d,\delta!) \in Sem(SE(\mathbb{G})^\delta))$ then $\sigma.(d,c@x)(d,\delta!).Sem(SE(\mathbb{G})^\delta))$

    on the other hand

If we note $tr$ the TC-transition that allowed the execution of $ev$ with $chan(tr)=chan(ev)$ (such transition exists by definition of ${\leadsto}_{\mathbb{TC}}$) then as the verdict is $\text{FAIL}^{dur}$, .i.e, $tgt(tr)=\text{FAIL}^{dur}$), we have (by rule $R9$) %$ev(ec)=c!y$ with $ec=src(tr)$ and $c=chan(ev)\in C^{out}$, and

\noindent $\begin{array}{rl}
     \phi(tr) = & f^{dur}(ec_1) \geq \maxWaitingBound \land  (\psi^{\delta}_{uspec} \land \psi^{obs}_{uspec} )\\    \psi^\delta_{uspec}=&\bigvee_{\substack{pec(ec')=ec_1 \\ chan(ec') \in C^{out}}} \exists f^{dur}(ec_1).\exists f^{out}_{chan(ec')} (ec_1).\exists F^{ini}.\pi(ec') \\
      \psi^{obs}_{uspec} = &   \bigwedge{\substack{pec(ec')=ec \\ chan(ec') \in C^{out}}} \forall F^{ini}.\forall f^{out}_{chan(ec')}.\neg\pi(ec') \\
      & \land \bigwedge_{\substack{pec(ec')=ec_1 \\ chan(ec') \in UC^{in}}} \forall F^{ini}. \forall f^{in}_{chan(ec')} . \neg \pi(ec')
\end{array}
$ 





$\nu'\models \phi(tr) $ thus $\nu' \models (\forall F^{ini}.\neg\pi(ec'))$ where $ec'$ as $ec'=pec(ec_1)$ and $chan(ec')\in C^{out}$ is the one among what figures in the conjunction of $ \phi(tr) $ (ii)

from (i) and (ii) we have contradiction thus $\sigma.ev\not\in Sem(SE(\mathbb{G})^\delta)$

\item $ec'=pec(ec_1)$ s.t. $\nu' \models \pi(ec_1) \land \bigwedge_{\substack{pec(ec')=ec_1\\ chan(ec')\in C^{out}}} .\forall f^{dur}(ec_1) .\forall f^{out}_{chan(ec')}(ec_1). \forall F^{ini}.\neg \pi(ec')$, $ev(ec')=ev=(z,\delta!)$ (quiescence enrichment def) 


$\nu'\models \phi(tr) $ thus $\nu' \models \bigvee_{\substack{pec(ec')=ec_1 \\ chan(ec') \in C^{out}}} \exists f^{dur}(ec_1).\exists f^{out}_{chan(ec')} (ec_1).\exists F^{ini}.\pi(ec')$  (ii)

from (i) and (ii) we have contradiction thus $\sigma.ev\not\in Sem(SE(\mathbb{G})^\delta)$

    
\end{itemize}






\end{itemize} 
