# Supplementary material for: Symbolic Path-guided Test Cases for Models with Data and Time
Source: arXiv:2309.06840 source file (2023-09-13)
Supplement: Supplementary file 4 [file proof_old1.tex]

\section{Proof of Th.~\ref{th:corr}}
\label{anx:proof}

\noindent We conduct the proof by using the contraposition principle. This means to prove that if there exists a test purpose $tp$ for $\mathbb{G}$ and a test case $\mathbb{TC}$ guided by $tp$ such that $\text{FAIL}^{out}$, $\text{FAIL}^{dur}\in vdt(LUT, \mathbb{TC})$ then $\neg(LUT~tioco~\mathbb{G})$. 

Based on the tioco definition, the non-conformance $\neg(LUT~tioco~\mathbb{G})$ amounts to prove that there exists $\sigma \in Sem(\mathbb{G}) \cap LUT$, and an $ev\in Evt(C^{out} \cup \{\delta\})$ such that : $\sigma.ev \in LUT$ and $\sigma.ev\not\in Sem(\mathbb{G})$. This is proved by the following proposition.

\begin{proposition}
\label{prop:corr}
If there exists a test purpose $tp$ for $\mathbb{G}$ and a test case $\mathbb{TC}$ guided by $tp$ such that $(\sigma.ev.\sigma',ec_0, \nu_0) ~\overset{*}{\leadsto}_{\mathbb{TC}} (\sigma',\emph{V}, \nu' )$ with $\emph{V} \in \{\emph{FAIL}^{out},\emph{FAIL}^{dur}\}$ then we have:
\begin{enumerate}

\item[{(1)}] $ev\in Evt(C^{out} \cup \{\delta\})$

\item[{(2)}] $\sigma \in Sem(\mathbb{G})\cap LUT$ 

\item[{(3)}] $\sigma.ev\in LUT$

\item[{(4)}] $\sigma.ev\not\in Sem(\mathbb{G})$
\end{enumerate}
\end{proposition}

{\bf{\em Proof of (1) from Prop.\ref{prop:corr}}} As  $(\sigma.ev.\sigma',ec_0, \nu_0) ~\overset{*}{\leadsto}_{\mathbb{TC}} (\sigma',\text{V}, \nu' )$ with $\text{V} \in \{\text{FAIL}^{out},\text{FAIL}^{dur}\}$, then there exists an execution step leading to $\text{FAIL}^{out}$ or $\text{FAIL}^{dur}$, i.e., $(\sigma.ev.\sigma',ec_0, \nu_0) \overset{*}{\leadsto}_{\mathbb{TC}} (ev.\sigma',ec,\nu){\leadsto}_{\mathbb{TC}} (\sigma',\text{V}, \nu' )$ such that the Test Case transition (TC-transition in short) $tr$ that allows the execution of $ev$ is inferred by rule $R5$ $\text{FAIL}^{out}$ or by rule $R10$ $\text{FAIL}^{dur}$. We additionally have $chan(tr)=chan(ev)$, and by hypothesis of $R5$ $\text{FAIL}^{out}$ resp. $R10$ $\text{FAIL}^{dur}$, $chan(tr) \in C^{out}$ resp. $chan(tr)=\delta$. We deduce that $ev\in Evt(C^{out} \cup \{\delta\})$.   

\medskip

{\bf{\em Proof of (2) from Prop.\ref{prop:corr}}} $\sigma \in LUT$ is a hypothesis as the execution relation ${\leadsto}_{\mathbb{TC}}$ applies on $LUT$ traces. Let us prove $\sigma \in Sem(\mathbb{G})$. 

As  $(\sigma.ev.\sigma',ec_0, \nu_0) ~\overset{*}{\leadsto}_{\mathbb{TC}} (\sigma',\text{V}, \nu' )$ with $\text{V} \in \{\text{FAIL}^{out},\text{FAIL}^{dur}\}$, we have that the last execution step until just before the consumption of $ev$ does not lead to a verdict, i.e. we have the decomposition $(\sigma.ev.\sigma',ec_0, \nu_0) ~\overset{*}{\leadsto}_{\mathbb{TC}} (ev.\sigma',ec, \nu ) \leadsto_{\mathbb{TC}} (\sigma',\text{V}, \nu' )$ where $ec$ is an execution context. This is because the TC-transition that allows the execution of $ev$ has as source an execution context and not a verdict by definition of rule $R5$ $\text{FAIL}^{our}$ or rule $R10\;\text{FAIL}^{dur}$. 

Furthermore, based on the execution steps and their correspondent TC-transitions, we have that any event of $\sigma$ is in $Evt(C)$, i.e., either of the form $(d,c!v)$ or $(d,c?v)$ and cannot be of the form $(d,\delta!)$. This is because there is no TC-transition $tr$ with target state being an execution context and $chan(tr)=\delta$. In fact, only rule $R9$ $\text{INC}^{dur}$ and rule $R10$ $\text{FAIL}^{dur}$ produce TC-transition on channel $\delta$ and their target state is a verdict.  



We have now to prove that if $(\sigma.ev.\sigma',ec_0,\nu_0) \overset{*}{\leadsto}_{\mathbb{TC}} ( ev.\sigma',ec, \nu )$ %with $q\not\in \mathbb{V}$,
then $\sigma \in Sem(\mathbb{G})$. 

Consider $\sigma= ev_1 \ldots ev_n$ with $ev_i\in Evt(C)$ for $i\in [1,n]$. It is sufficient to prove that if $(ev_1.ev_2\ldots ev_n.ev.\sigma',ec_0,\nu_0) %\leadsto_{\mathbb{TC}} (ev_2.\ldots ev_n.ev.\sigma',ec_1,\nu_1) 
\ldots \leadsto_{\mathbb{TC}} (ev_n.ev.\sigma',ec_{n-1},\nu_{n-1}) \leadsto_{\mathbb{TC}} ( ev.\sigma',ec_n, \nu_n )$ where $ec$ and $\nu$ are denoted by resp. $ec_n$ and $\nu_n$ for clarity in what follows, then there exists an underlying path of the form $p=ec_0.ec_1\ldots ec_n$ such that $M \models_{\nu_n} \exists F^{ini}.\pi(ec_n)$ and $\nu_n(p)=\sigma$. This implies that $\sigma\in Traces(\mathbb{G})$, and thus $\sigma \in Sem(\mathbb{G})$. We show this by induction on the size of $\sigma$.

\medskip 

\noindent Case $\sigma$ of size $1$, i.e., $\sigma=ev_1$ with $ev_1$ is an event, given $(ev_1.ev.\sigma',ec_0,\nu_0) \leadsto_{\mathbb{TC}} (ev.\sigma',ec_1, \nu_1 )$, we show that there exists an underlying path of the form $p_1=ec_0.ec_1$ such that $M \models_{\nu_1} \exists F^{ini}.\pi(ec_1)$ and $\nu_1(p_1)=\sigma$.

%$ev_1\in Sem(\mathbb{G})$:

\begin{itemize}
    \item Case $ev_1=(d,c!v)$: If we note $tr$ the TC-transition that allows the execution of $ev_1$ with $chan(tr)=c$ (such transition exists by definition of $\leadsto_{\mathbb{TC}}$) then we have: $tgt(tr)=ec_1$; $ev(ec_1)=(z,c!y)$ with $z=f ^{dur}(ec_0)$ and $y=f^{out}_c(ec_0)$; $pec(ec_1)=ec_0$; and

    \medskip
    
    $\phi(tr) = (z < \maxWaitingBound) \land (\exists F^{ini}.\pi( ec_1 ) ) $  
    
    \hfill(by rule $R2\;\text{SKIP}$).

    \medskip 

   On the other hand $M \models_{\nu_1}  \phi(tr)$ where $\nu_1=\nu_0[z \mapsto d][y\mapsto v]$ (by definition  $\leadsto_{\mathbb{TC}}$) then $M \models_{\nu_1} \exists F^{ini}.\pi( ec_1 )$ ($\nu_1$ satisfies the right-side of the conjunction of $\phi(tr)$). We can thus compute a trace for the path $p_1=ec_0ec_1$ (a path indeed because $pec(ec_1)=ec_0$)
   using $\nu_1$, i.e. $\nu_1(p_1)=\nu_1(ev(ec_0)).\nu_1(ev(ec_1) )$ which is $(\nu_1(z),c!\nu_1(y))=(d,c!v)$ equals $ev_1$ (by convention $\nu_1(ev(ec_0))=\epsilon$ as $ec_0$ is the initial context in $p_1$). We conclude that $ev_1\in Traces(\mathbb{G})$ and hence $ev_1 \in Sem(\mathbb{G})$.

\medskip 

    \item Case $ev_1=(d,c?v)$ with $c\in UC^{in}$, similar to $ev_1=(d,c!v)$: If we note $tr$ the TC-transition that allows the execution of $ev_1$ with $chan(tr)=c$ (such transition exists by definition of $\leadsto_{\mathbb{TC}}$) then we have: $tgt(tr)=ec_1$; $ev(ec_1)=(z,c?x)$ with $z=f ^{dur}(ec_0)$ and $y=f^{in}_c(ec_0)$; $pec(ec_1)=ec_0$; and

    \medskip
    
    $\phi(tr) = (z < \maxWaitingBound) \land (\exists F^{ini}.\pi( ec ) ) $  
    
    \hfill(by rule $R6\;\text{SKIP}$).

    \medskip 

   On the other hand $M \models_{\nu_1}  \phi(tr)$ where $\nu_1=\nu_0[z \mapsto d][x\mapsto v]$ (by definition  $\leadsto_{\mathbb{TC}}$) then $M \models_{\nu_1} \exists F^{ini}.\pi( ec_1 )$ ($\nu_1$ satisfies the right-side of the conjunction of $\phi(tr)$). We can thus compute a trace for the path $p_1=ec_0ec_1$ (a path indeed because $pec(ec_1)=ec_0$)
   using $\nu_1$, i.e. $\nu_1(p_1)=\nu_1(ev(ec_0)).\nu_1(ev(ec_1) )$ which is $(\nu_1(z),c?\nu_1(x))=(d,c?v)$ equals $ev_1$ (by convention $\nu_1(ev(ec_0))=\epsilon$ as $ec_0$ is the initial context in $p_1$). We conclude that $ev_1\in Traces(\mathbb{G})$ and hence $ev_1 \in Sem(\mathbb{G})$.

\medskip 

%STIM
     \item Case $ev_1=(d,c?v)$ with $c\in CC^{in}$: If we note $tr$ the TC-transition that allows the execution of $ev_1$ with $chan(tr)=c$ (such transition exists by definition of $\leadsto_{\mathbb{TC}}$) then we have: $tgt(tr)=ec_1$; $ev(ec_1)=(z,c?x)$ with $z=f ^{dur}(ec_0)$ and $y=f^{in}_c(ec_0)$; $pec(ec_1)=ec_0$; and

    \medskip
    
        $\phi(tr)=\exists (F^{ini} \cup Var(\pi(tp)) ) \setminus \overline{f}(ec_1). \pi(tp) $
    
    \hfill(by rule $R1\;\text{SKIP}$).

    \medskip 

   On the other hand $M \models_{\nu_1}  \phi(tr)$ where $\nu_1=\nu[z \mapsto d][x\mapsto v]$ (by definition  $\leadsto_{\mathbb{TC}}$). Given $ec_1$ is a context of the test purpose $tp$, hence its path condition $\pi(ec_1)$ is in conjunction some other constraints accumulated until the computation of $tgt(tp)$ (by the definition of symbolic execution) then 
   
   $M \models_{\nu_1} \exists (F^{ini} \cup Var(\pi(tp)) ) \setminus \overline{f}(ec_1).\pi( ec_1 )$. We have also that $\nu_1$ satisfies $\pi(ec_1)$ for the values $d$ resp. $v$  associated with $f^{dur}(ec_0)$ resp. $f^{in}_c(ec_0)$ through $\nu_1$ because these variables are excluded from the variables which are bound by the existential quantifier in the expression of $\phi(tr)$ ($f^{dur}(ec_0)$, $f^{in}_c(ec_0) \in \overline{f}(ec_1)$). Given that variables of $Var(tp)$ other than $f^{dur}(ec_0)$, $f^{in}_c(ec_0)$, can be equally considered to be bound or not bound by the existential quantifier in the previous satisfaction statement through $\nu_1$, we have that $M \models_{\nu_1} \exists F^{ini}.\pi( ec_1 )$. We can thus compute a trace for the path $p=ec_0ec_1$ (a path indeed because $pec(ec_1)=ec_0$) using $\nu_1$, i.e. $\nu_1(p_1)=\nu_1(ev(ec_0)).\nu_1(ev(ec_1) )$ which is $(\nu_1(z),c?\nu_1(x))=(d,c?v)$ equals $ev_1$. We conclude that $ev_1\in Traces(\mathbb{G})$ and hence $ev_1 \in Sem(\mathbb{G})$.

    
\end{itemize}
 

\medskip


\noindent Induction case on size of $\sigma$ greater than $1$, i.e., $\sigma= ev_1 \ldots ev_n$ with $ev_i\in Evt(C)$ for $i\in [1,n]$, we prove that if $(ev_1.ev_2\ldots ev_n.ev.\sigma',ec_n,\nu_n) %\leadsto_{\mathbb{TC}} (ev_2.\ldots ev_n.ev.\sigma',ec_1,\nu_1) 
\ldots \leadsto_{\mathbb{TC}} (ev_n.ev.\sigma',ec_{n-1},\nu_{n-1}) \leadsto_{\mathbb{TC}} ( ev.\sigma',ec_n, \nu_n )$ then there exists an underlying path of the form $p_n=ec_0.ec_1 \ldots ec_n$ with $ec_n$ such that $M \models_{\nu_n} \exists F^{ini}.\pi(ec_n)$ and $\nu_{n}(p_n)=\sigma$.


\begin{itemize}

\item Case $ev_n=(d,c!v)$:  If we note $tr$ the TC-transition that allows the execution of $ev_n$ with $chan(tr)=c$ (such transition exists by definition of $\leadsto_{\mathbb{TC}}$) then we have: $tgt(tr)=ec_n$; $ev(ec_n)=(z,c!y)$ with $z=f ^{dur}(ec_{n-1})$ and $y=f^{out}_c(ec_{n-1})$ where $pec(ec_n)=ec_{n-1}$; and
    \medskip
    
    $\phi(tr) = (z < \maxWaitingBound) \land (\exists F^{ini}.\pi( ec_n ) ) $  
    
    \hfill(by rule $R2\;\text{SKIP}$).

    \medskip 

    By the induction hypothesis, there exists an underlying path of the form $p_{n-1}=ec_0.ec_1.\ldots.ec_{n-1}$ such that $M \models_{\nu_{n-1}} \exists F^{ini}.\pi(ec_{n-1})$ and $\nu_{n-1}(p_{n-1})=ev_1\ldots ev_{n-1}$. On the other hand $M \models_{\nu_n}  \phi(tr)$ where $\nu_n=\nu_{n-1}[z \mapsto d][y\mapsto v]$ (by definition of $\leadsto_{\mathbb{TC}}$) then $M \models_{\nu_n} \exists F^{ini}.\pi( ec_n )$ ($\nu_n$ satisfies the right-side of the conjunction of $\phi(tr)$). We can thus compute a trace for the path $p_n=ec_0.ec_1 \ldots ec_{n-1}.ec_n$ (a path indeed because $pec(ec_n)=ec_{n-1}$) using $\nu_n$, i.e. $\nu_n(p_n)=\nu_n(p_{n-1}).\nu_n( ev(ec_n) )$ with $\nu_n(p_{n-1})=\nu_n( ev(ec_0) ) \ldots \nu_n( ev(ec_{n-1}))$. As $\nu_n$ coincide with $\nu_{n-1}$ on all fresh variables used to evaluate $ev(ec_i)$ for $i\in [1,n-1]$ ($z$ and $y$ are fresh variables introduced later and used to evaluate $ev(ec_n)$), we have $\nu_n(p_{n-1})=\nu_{n-1}(p_{n-1})$ equals $ev_1\ldots ev_{n-1}$. Furthermore, $\nu_n(ev(ec_n))=(\nu_n(z),c!\nu_n(y))=(d,c!v)$ equals $ev_n$. Thus, $\nu_n(p_n)=ev_1 \ldots ev_{n-1}.ev_n$ equals $\sigma$. We conclude that $\sigma\in Traces(\mathbb{G})$ and hence $\sigma \in Sem(\mathbb{G})$.
 

\medskip 

\item Cases $ev_n=(d,c?v)$ with $c\in UC^{in}$ and $ev_n=(d,c?v)$ with $c\in CC^{in}$ are similar to the previous case by considering resp. rule $R6$ $\text{SKIP}$ and $R1$ $\text{SKIP}$. As for previous case of $ev_n=(d,c!v)$, the reasoning uses the arguments of the base case of induction transposed to $ev_n$.
\end{itemize}

\medskip

{\bf{\em Proof of (3) from Prop.\ref{prop:corr}}} $\sigma.ev \in LUT$ is a hypothesis as the execution relation ${\leadsto}_{\mathbb{TC}}$ applies on $LUT$ traces.

\medskip

{\bf{\em Proof of (4) from Prop.\ref{prop:corr}}} Given the execution $(\sigma.ev.\sigma',ec_0, \nu_0) ~\overset{*}{\leadsto}_{\mathbb{TC}} (\sigma',\text{V}, \nu' )$ with $\text{V} \in \{\text{FAIL}^{out},\text{FAIL}^{dur}\}$, we prove that $\sigma.ev\not\in Sem(\mathbb{G})$. We will argue for each case of the executions that lead to $\text{FAIL}^{out}$ and $\text{FAIL}^{dur}$.   

\begin{itemize}
   
\item Case of decomposition $(\sigma.ev.\sigma',ec_0, \nu_0) ~\overset{*}{\leadsto}_{\mathbb{TC}} (ev.\sigma',ec, \nu ) {\leadsto}_{\mathbb{TC}} (\sigma',\text{FAIL}^{out}, \nu' )$:

By {\bf{\em (1) from Prop.\ref{prop:corr}}}, 
we have that $ev$ is of the form $(d,c!v)$. By {\bf{\em (2) from Prop.\ref{prop:corr}}}, we have that  $\sigma \in Sem(\mathbb{G})$. Furthermore, we have that there exists an underlying path $p$ such that $tgt(p)=ec$, $\nu \models \exists F^{ini}.\pi(ec)$ and $\nu(p)=\sigma$. Now if we note $tr$ the TC-transition that allows the execution of $ev$, we have $chan(tr)=chan(ev)$, $src(tr)=ec$ (such transition exists by definition of ${\leadsto}_{\mathbb{TC}}$), as the verdict is $\text{FAIL}^{out}$, we have $tgt(tr)=\text{FAIL}^{out}$; and 

\medskip

\noindent $\begin{array}{l}
     \phi(tr) =  (f^{dur} (ec)  < \maxWaitingBound )   \land  \bigwedge_{\substack{pec(ec') =ec \\ chan(ec')=c }}(\forall F^{ini}.\neg\pi(ec'))
\end{array}
$ 

 \hfill(by rule $R5\;\text{FAIL}^{out}$).

 %On the other hand $M \models_{\nu_1}  \phi(tr)$ where $\nu_1=\nu[z \mapsto d][x\mapsto v]$ (by definition  $\leadsto_{\mathbb{TC}}$)


On the other hand $\nu'\models \phi(tr) $ with $\nu'=\nu[f^{dur}(ec)\mapsto d][f^{out}_c(ec) \mapsto v]$ thus $\nu' \models \forall F^{ini}.\neg\pi(ec')$ for any successor $ec'$ of $ec$ ($pec(ec')=ec$) such that $chan(ec')=c$. That is, for any such successor $ec'$, $\nu' \not\models \exists F^{ini}.\pi(ec')$. Thus, there is no $ec'$ which extends $p$ into a path $p.ec'$ carrying $\sigma.ev$ through $\nu'$, i.e., such that $\nu' \models \exists F^{ini}.\pi(ec')$ and $\nu'(p.ec')=\sigma.ev$. We conclude that $\sigma.ev\not\in Traces(\mathbb{G})$. As $Sem(\mathbb{G})$ contains $Traces(\mathbb{G})$ together with strict prefixes from $Traces(\mathbb{G})$ completed with quiescence observation, i.e., ending with events of the form $(d,\delta!)$, and given $ev=(d,c!v)$ is not such event, we have $\sigma.ev\not\in Sem(\mathbb{G})$.


%case FAIL_dur
\item Case of decomposition $(\sigma.ev.\sigma',ec_0, \nu_0) ~\overset{*}{\leadsto}_{\mathbb{TC}} (ev.\sigma',ec, \nu ) {\leadsto}_{\mathbb{TC}} (\sigma',\text{FAIL}^{dur}, \nu' )$:

By {\bf{\em (1) from Prop.\ref{prop:corr}}}, 
we have that $ev$ is of the form $(d,\delta!)$. By {\bf{\em (2) from Prop.\ref{prop:corr}}}, we have that  $\sigma \in Sem(\mathbb{G})$. Furthermore, we have that there exists an underlying path $p$ such that $tgt(p)=ec$, $\nu \models \exists F^{ini}.\pi(ec)$ and $\nu(p)=\sigma$. Now if we note $tr$ the TC-transition that allows the execution of $ev$, we have $chan(tr)=chan(ev)$, $src(tr)=ec$ (such transition exists by definition of ${\leadsto}_{\mathbb{TC}}$), as the verdict is $\text{FAIL}^{dur}$, we have $tgt(tr)=\text{FAIL}^{dur}$; and 

\medskip

\noindent $\begin{array}{l}
      \phi(tr) = f^{dur}(ec) \geq \maxWaitingBound
    \land \bigwedge_{\substack{pec(ec')=ec 
        \\ chan(ec') \in C^{out} \cup UC^{in} \cup \{\delta\}}} \forall F^{ini}.\neg \pi(ec')
\end{array}
$ 

 \hfill(by rule $R10\;\text{FAIL}^{dur}$).
 
On the other hand $\nu'\models \phi(tr) $ with $\nu'=\nu[f^{dur}(ec)\mapsto d]$ thus $\nu' \models \forall F^{ini}.\neg\pi(ec')$ for any successor $ec'$ of $ec$ ($pec(ec')=ec$) such that $chan(ec')\in C^{out} \cup UC^{in} \cup \{\delta\}$. We consider two cases: $chan(ec')=\delta!$ and $chan(ec')\in C^{out} \cup UC^{in}$. In the first case $chan(ec')=\delta!$, there is at most one of such successor $ec'$ by the quiescence enrichment. Yet as $\nu' \not\models \exists F^{ini}.\pi(ec')$, we cannot extend $p$ into a path $p.ec'$ carrying $\sigma.ev$ through $\nu'$, i.e., such that $\nu' \models \exists F^{ini}.\pi(ec')$ and $\nu'(p.ec')=\sigma.ev$. We conclude that $\sigma.ev\not\in Traces(\mathbb{G})$. Let us examine now the case $chan(ec')\in C^{out} \cup UC^{in}$. Those successors $ec'$ can result in traces ending with quiescence observation in $Sem(\mathbb{G})$. Such quiescent traces are of the form $\sigma.(d',\delta!)$ with $d'< d$ and are carried by $p.ec'$ through $\nu_1$, i.e., such that $\nu' \models \exists F^{ini}.\pi(ec')$ and $\nu'(p.ec')=\sigma.(d,c!v)$ or $\nu'(p.ec')=\sigma.(d,c?v)$ with $c=chan(ec')$. Yet as $\nu' \not\models \exists F^{ini}.\pi(ec')$, we cannot infer such traces in $Sem(\mathbb{G})$. We conclude that $\sigma.ev\not\in Sem(\mathbb{G})$.
\qed





\end{itemize} 
